# Supplementary material for: Data-efficient Fine-tuning for LLM-based Recommendation
Source: arXiv:2401.17197 source file (2024-06-04)
Supplement: Supplementary file 1 [file 6_SI.tex]

\section{Appendix}\label{sec:appendix}
